# Supplementary material for: Measurement of ZZ production in pp collisions at sqrt(s)=7 TeV and limits on anomalous ZZZ and ZZgamma couplings with the ATLAS detector
Source: arXiv:1211.6096 source file (2012-11-26)
Supplement: Supplementary file 1 [file AppendixPlots.tex]

\section {Auxiliary plots to be shown in conferences} 

Cross section comparison with previous measurements.

 \begin{figure}[htbp]
 \begin{center}
  \includegraphics[width=0.5\textwidth]{figures/SigmaZZatNLO}\hfill
  \caption{\small \label{fig:xseccomb}
 Comparison of experimental measurements and theoretical predictions of the total \ZZ\ production cross section as a
 function of centre of mass energy $\sqrt{s}$. Shown are experimental
 measurements from CDF and D0 in
 $p\bar{p}$ collisions at the Tevatron at $\sqrt{s} = 1.96$~TeV, and
 experimental measurements from ATLAS in $pp$
 collisions at the LHC at $\sqrt{s} = 7$~TeV  and $\sqrt{s} = 8$~TeV (https://cdsweb.cern.ch/record/1460409). The blue
 dashed line shows the theoretical prediction for the \ZZ\ production cross section in $p\bar{p}$
 collisions, calculated at NLO in QCD using
 MCFM with PDF set CT10. The
 solid red line shows the theoretical prediction for  the \ZZ\ production cross
 section in $pp$ collisions, calculated in the same way.
 The theoretical curves assume the zero-width approximation.
   }
 \end{center}
 \end{figure}

\newpage
Unfolding plots using a fixed bin width.

\begin{figure}[htbp]
\begin{center}
\subfigure[]{\includegraphics[width=0.48\textwidth]{figures/ZZllll_ZpT_UnfoldedDistribution}}
\subfigure[]{\includegraphics[width=0.48\textwidth]{figures/ZZllnn_ZpT_UnfoldedDistribution}}
\caption{\label{fig:unfolded_fixed}Normalized and unfolded $ZZ$ fiducial cross sections in bins of the \pT\ of the leading $Z$ boson for (a) the \zzllll\ selection and (b) the \zzllvv\ selection.}
\end{center}
\end{figure}

\begin{figure}[htbp]
\begin{center}
\subfigure[]{\includegraphics[width=0.48\textwidth]{figures/ZZllll_DPhiLep_UnfoldedDistribution}}
\subfigure[]{\includegraphics[width=0.48\textwidth]{figures/ZZllnn_DPhiLep_UnfoldedDistribution}}
\caption{\label{fig:unfoldedDphi_fixed}Normalized and unfolded $ZZ$ fiducial cross sections in bins of the $\Delta\phi(\ell,\ell')$ of the leading $Z$ boson for (a) the \zzllll\ selection and (b) the \zzllvv\ selection.}
\end{center}
\end{figure}

\begin{figure}[htbp]
\begin{center}
\subfigure[]{\includegraphics[width=0.48\textwidth]{figures/ZZllll_ZZTMass_UnfoldedDistribution}}
\subfigure[]{\includegraphics[width=0.48\textwidth]{figures/ZZllnn_ZZTMass_UnfoldedDistribution}}
\caption{\label{fig:unfoldedM4l_fixed}Normalized and unfolded $ZZ$ fiducial cross sections in bins of $m^{ZZ}$ for the (a) \zzllll\ selection and of $m^{ZZ}_{T}$ for the (b) \zzllvv\ selection.}
\end{center}
\end{figure}

The unfolded \ZZ\ fiducial cross sections together with the correlation coefficients between the different analysis bins are shown in tables~\ref{tab:correlation_pT_4l} to~\ref{tab:correlation_mT_2l2n}.

\begin{table}
  \centering
  \begin{tabular}{lrrrr}
    \hline
    Leading $Z$ boson \pT\ (GeV)                                                           & [0,60] & [60,100] & [100,200] & [200,600]  \\
    \hline
    1 / $\sigma^{\rm fid}_{ZZ}$ d $\sigma^{\rm fid}_{ZZ}$ / d \pT\ $Z$      & 0.0070       &  0.0098      & 0.0016      & 0.00005 \\
    Relative Uncertainty                                                              & 15.7 \%  & 16.6 \%  & 30.4 \% &  74.2 \%  \\
    \hline
    Correlation                                                                            &    1         & -0.70     & -0.36   & -0.11  \\
                                                                                                  &               & 1            & -0.34  & -0.13  \\
                                                                                                  &               &                & 1        & -0.06  \\                                                                                                  &               &                &           & 1      \\
   \hline
   \end{tabular}
   \caption{\label{tab:correlation_pT_4l}
Unfolded fiducial cross section together with the overall uncertainty in bins of the leading $Z$ \pT\ for the 
\zzllll\ selection. The correlation coefficients between 
different leading $Z$ \pT\ bins are also shown. Half of the symmetric correlation matrix is presented. }
\end{table}

\begin{table}
  \centering
  \begin{tabular}{lrrr}
    \hline
    Leading $Z$ boson \pT\ (GeV)                                                          & [50,90] & [90,130] & [130,200]   \\
    \hline
    1 / $\sigma^{\rm fid}_{ZZ}$ d $\sigma^{\rm fid}_{ZZ}$ / d \pT\ $Z$      & 0.0099           & 0.0083       & 0.0039            \\
    Relative Uncertainty                                                               & 34.5\%      & 38.9\%   & 39.5\%  \\
    \hline
    Correlation                                                                             & 1      & -0.67  & -0.46  \\
                                                                                                  &        &        1    & -0.33  \\
                                                                                                  &        &             & 1      \\

   \hline
   \end{tabular}
   \caption{\label{tab:correlation_pT_2l2n}
Unfolded fiducial cross section together with the overall uncertainty in bins of the leading $Z$ \pT\ for the 
\zzllvv\ selection. The correlation coefficients between different leading $Z$ \pT\ bins are also shown. 
Half of the symmetric correlation on matrix is presented. }
\end{table}

\begin{table}
  \centering
  \begin{tabular}{lrrrr}
    \hline
    $\Delta\phi(\ell^+,\ell^- )$                                                                              & [0,0.5]        & [0.5,1.0]          & [1.0,1.7]        & [1.7,$\pi$]   \\
    \hline
    1 / $\sigma^{\rm fid}_{ZZ}$ d $\sigma^{\rm fid}_{ZZ}$ / d $\Delta\phi(\ell^+,\ell^- )$     & 0.12            & 0.28             & 0.26             & 0.43             \\
    Relative Uncertainty                                                                                          & 53.4\%   & 34.7\%   & 30.3\%   & 11.1\%  \\
    \hline
    Correlation                                                                                                        &  1      & -0.15  & -0.07  & -0.32  \\
                                                                                                                             &           & 1        & -0.16  & -0.47  \\
                                                                                                                             &           &           &  1        & -0.62  \\
                                                                                                                             &           &           &            & 1      \\

   \hline
   \end{tabular}
   \caption{\label{tab:correlation_Dphi_4l}
Unfolded fiducial cross section together with the overall uncertainty in bins of the $\Delta\phi(\ell^+,\ell^- )$ of the leading $Z$ boson for the \zzllll\ selection. The correlation coefficients between different $\Delta\phi(\ell^+,\ell^- )$ of the leading $Z$ \pT\ bins are also shown. Half of the symmetric correlation matrix is presented. }
\end{table}

\begin{table}
  \centering
  \begin{tabular}{lrrrr}
    \hline
    $\Delta\phi(\ell^+,\ell^- )$                                                                               & [0,0.5]        & [0.5,1.7]        & [1.7,$\pi$]       \\
    \hline
    1 / $\sigma^{\rm fid}_{ZZ}$ d $\sigma^{\rm fid}_{ZZ}$ / d $\Delta\phi(\ell^+,\ell^- )$      & 0.35            & 0.57             & 0.10            \\
    Relative Uncertainty                                                                                           & 46.0\%   & 20.3\%   &  90.7\%  \\
    \hline
    Correlation                                                                                                        &  1      & -0.38  & -0.19  \\
                                                                                                                             &          & 1         & -0.82  \\
                                                                                                                             &          &            & 1      \\

   \hline
   \end{tabular}
   \caption{\label{tab:correlation_Dphi_2l2n}
Unfolded fiducial cross section together with the overall uncertainty in bins of the $\Delta\phi(\ell^+,\ell^- )$  of the
leading $Z$ boson for the \zzllvv\ selection. The correlation coefficients between different $\Delta\phi(\ell^+,\ell^- )$ bins of the
leading $Z$ boson are also shown. Half of the symmetric correlation matrix is presented. }
\end{table}

\begin{table}
  \centering
  \begin{tabular}{lrrrr}
    \hline
    $m_{ZZ}$ (GeV)                                                                       & [0,240]        & [240,300]        & [300,400]        & [400,800]       \\
    \hline
    1 / $\sigma^{\rm fid}_{ZZ}$ d $\sigma^{\rm fid}_{ZZ}$ / d $m_{ZZ}$      & 0.0021             & 0.0045             & 0.0010             & 0.00028             \\
    Relative Uncertainty                                                              & 13.2\%         & 23.1\%         & 39.8\%         & 37.5\%  \\
    \hline
    Correlation                                                                             &   1      & -0.65  & -0.26  & -0.37  \\
                                                                                                   &   & 1      & -0.24  & -0.17  \\
                                                                                                   &  &  & 1      & -0.16  \\
                                                                                                   &  &  &  & 1      \\

   \hline
   \end{tabular}
   \caption{\label{tab:correlation_m_4l}
Unfolded fiducial cross section together with the overall uncertainty in bins of $m^{ZZ}$ for the \zzllll\ selection. The correlation coefficients between different $m^{ZZ}$ bins are also shown. Half of the symmetric correlation matrix is presented. }
\end{table}

\begin{table}
  \centering
  \begin{tabular}{lrrrr}
    \hline
    $m_{\rm T}$ (GeV)                                                                       & [220,250]        & [250,300]        & [300,400]       \\
    \hline
    1 / $\sigma^{\rm fid}_{ZZ}$ d $\sigma^{\rm fid}_{ZZ}$ / d $m_{\rm T}$       & 0.011             & 0.0063             & 0.0037             \\
    Relative Uncertainty                                                                                          & 45.7\%   & 42.0\%   & 35.2\%  \\
    \hline
    Correlation                                                                                                        &  1      & -0.56  & -0.53   \\
                                                                                                                             &          & 1         & -0.39  \\
                                                                                                                             &          &            & 1      \\

   \hline
   \end{tabular}
   \caption{\label{tab:correlation_mT_2l2n}
Unfolded fiducial cross section together with the overall uncertainty in bins of $m^{ZZ}_{T}$ for the \zzllvv\ selection. The correlation coefficients between different  $m^{ZZ}_{T}$ bins are also shown. Half of the symmetric correlation matrix is presented. }
\end{table}

  \newpage
  Transverse momentum of leading \Z\ with fine bins (20 GeV), for the \zzllll\ and the \zzsllll\ selections.
 
  \begin{figure}[htbp]
  \begin{center}
  \subfigure[]{
  \includegraphics[width=0.47\textwidth]{figures/h_4l_ZZ_Z1_pt}
  }
  \subfigure[]{
  \includegraphics[width=0.47\textwidth]{figures/h_4l_ZZs_Z1_pt}
  }
  \caption{\label{fig:ptLeadingZ_finebin}Transverse momentum $\pT^{Z}$ of the leading \Z\ for (a) the \zzllll\ and (b) the \zzsllll\ selection.  The points represent the observed data and the
  histograms show the prediction from simulation, 
  where the background is normalized to the data-driven (dd) estimate. The shaded band
  shows the combined statistical and systematic uncertainty on the prediction.
  The shaded band shows the combined statistical and systematic uncertainty on the signal prediction.
  }
  \end{center}
  \end{figure}
